# Supplementary material for: CCCL: Node-Spanning GPU Collectives with CXL Memory Pooling
Source: arXiv:2602.22457 source file (2026-05-06)
Supplement: Supplementary file 1 [file Appendix_math_.tex]

% \section{Appendix: Mathematical Framework and ADMM Algorithm}

% The TV-regularized laminography reconstruction problem is initially formulated as follows:

% \begin{align}
% & \min_{u} \frac{1}{2}|| L u - d ||_2^2 + \lambda ||  \psi ||_{\text{TV}} \quad \text{S.T.} \quad \nabla u = \psi \tag{1}
% \end{align}

% This optimization problem combines a data fidelity term with Total Variation regularization, subject to the constraint that $\psi$ equals the gradient of u. To solve this constrained optimization problem, we construct the augmented Lagrangian:

% \begin{align}
%     & \mathcal{L}_\rho(\psi,u,\lambda) = \|Lu - d\|_2^2 + \alpha\|\psi\|_1 + \notag  \\ &
%  2\text{Re}\{\lambda^H(\nabla u - \psi)\} + \rho\|\nabla u - \psi\|_2^2 \tag{2}
% \end{align}

% The augmented Lagrangian includes the original objective function terms, adds a Lagrangian term with multiplier $\lambda$, and includes a quadratic penalty term with parameter $\rho$. The ADMM algorithm then alternates between three update steps. 

% First, we update $u$ while keeping $\psi$ and $\lambda$ fixed, and this problem is attributed to the \textbf{LSP}:

% \begin{align}
% u^{k+1}=\arg\min_u \mathcal{L}_\rho(\psi^k,u,\lambda^k) \tag{3}
% \end{align}

% This subproblem can be reformulated as follows:

% \begin{align}
% \min_u \|Lu-d\|_2^2+\rho\|\nabla u-\psi +\frac{\lambda}{\rho}\|_2^2\tag{4}
% \end{align}

% This is solved using the conjugate gradient method.

% Next, we update the auxiliary variable $\psi$ using the new $u$ value while keeping $\lambda$ fixed, which is attributed to the \textbf{RSP}:

% \begin{align}
% \psi^{k+1}=\arg\min_\psi \mathcal{L}_\rho(u^{k+1},\psi,\lambda^k) \tag{5}
% \end{align}

% This subproblem has a closed-form solution involving a soft thresholding operation:

% \begin{align}
% \tilde{\psi}=\frac{\nabla u+\lambda/\rho}{|\nabla u+\lambda/\rho|}\max(0,|\nabla u+\lambda/\rho|-\alpha/\rho)\tag{6}
% \end{align}

% Finally, we update the Lagrange multiplier $\lambda$ using the new values of $u$ and $\psi$:

% \begin{align}
% \lambda^{k+1}=\lambda^k+\rho(u^{k+1}-\psi^{k+1})\tag{7}
% \end{align}
